# Supplementary material for: Atomic electronic structure calculations with Hermite interpolating polynomials
Source: arXiv:2302.00440 ancillary file (2023-04-26)
Supplement: Supplementary file 1 [file suppinfo.pdf]

# Supporting Information: Atomic Electronic Structure Calculations with Hermite Interpolating Polynomials

Susi Lehtola<sup>\*,†,‡</sup>

<sup>†</sup>*Molecular Sciences Software Institute, Blacksburg, Virginia 24061, United States*

<sup>‡</sup>*Department of Chemistry, University of Helsinki, P.O. Box 55, FI-00014 University of Helsinki, Finland*

E-mail: susi.lehtola@alumni.helsinki.fi

The convergence of the Taylor expansion of the basis functions near the nucleus is shown in figure S1 for a 15-node LIP basis and figure S2 for an 8-node HIP basis, both with 5 radial elements. The case for 25 radial elements is shown in figures S3 and S4, respectively.

The plots for  $\tau$  and  $\nabla^2 n$  for the studied functionals from the calculations employing five radial elements and the high-order numerical basis sets are shown in

- figure S5 for the HF calculation
- figure S6 for the TPSS calculation
- figure S7 for the TASKCC calculation
- figure S8 for the M05 calculation
- figure S9 for the M06 calculation
- figure S10 for the M06-SX calculation
- figure S11 for the M06-L calculation
- figure S12 for the revM06 calculation
- figure S13 for the revM06-L calculation
- figure S14 for the M08-SO calculation
- figure S15 for the M08-HX calculation
- figure S16 for the M11 calculation
- figure S17 for the revM11 calculation
- figure S18 for the M11-L calculation
- figure S19 for the MN12-SX calculation
- figure S20 for the MN12-L calculation
- figure S21 for the MN15 calculation
- figure S22 for the MN15-L calculation
- figure S23 for the  $\omega$ B97X-noV calculation
- figure S24 for the B97M-noV calculation
- figure S25 for the  $\omega$ B97M-noV calculation
- figure S26 for the r<sup>2</sup>SCAN calculation

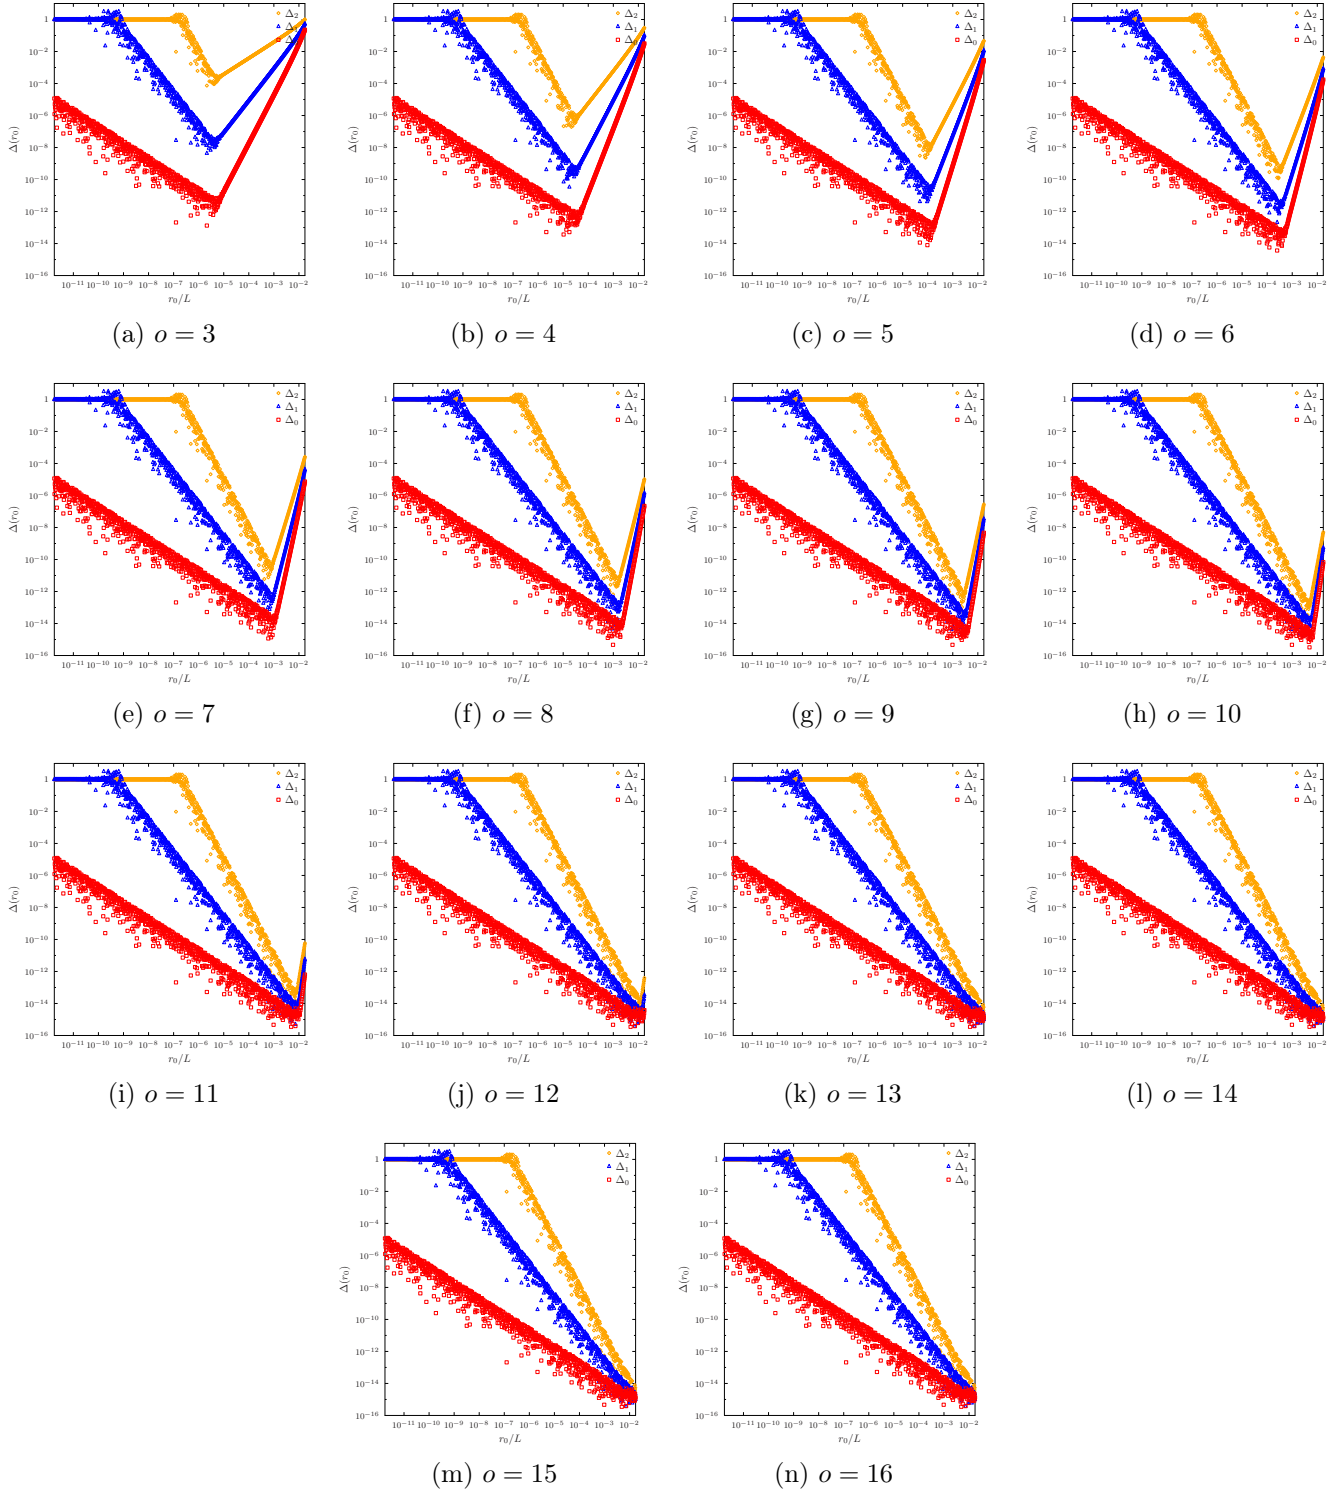

Figure S1: Error  $\Delta$  in Taylor expansion as a function of the switching radius  $R$  for various orders  $o$  of the Taylor expansion, for a 15-node LIP basis with 5 elements; the first non-nuclear node is at  $r_2/L \approx 0.017377$ . Convergence is reached at  $o = 14$ , matching the polynomial order of the 15-node LIP basis.

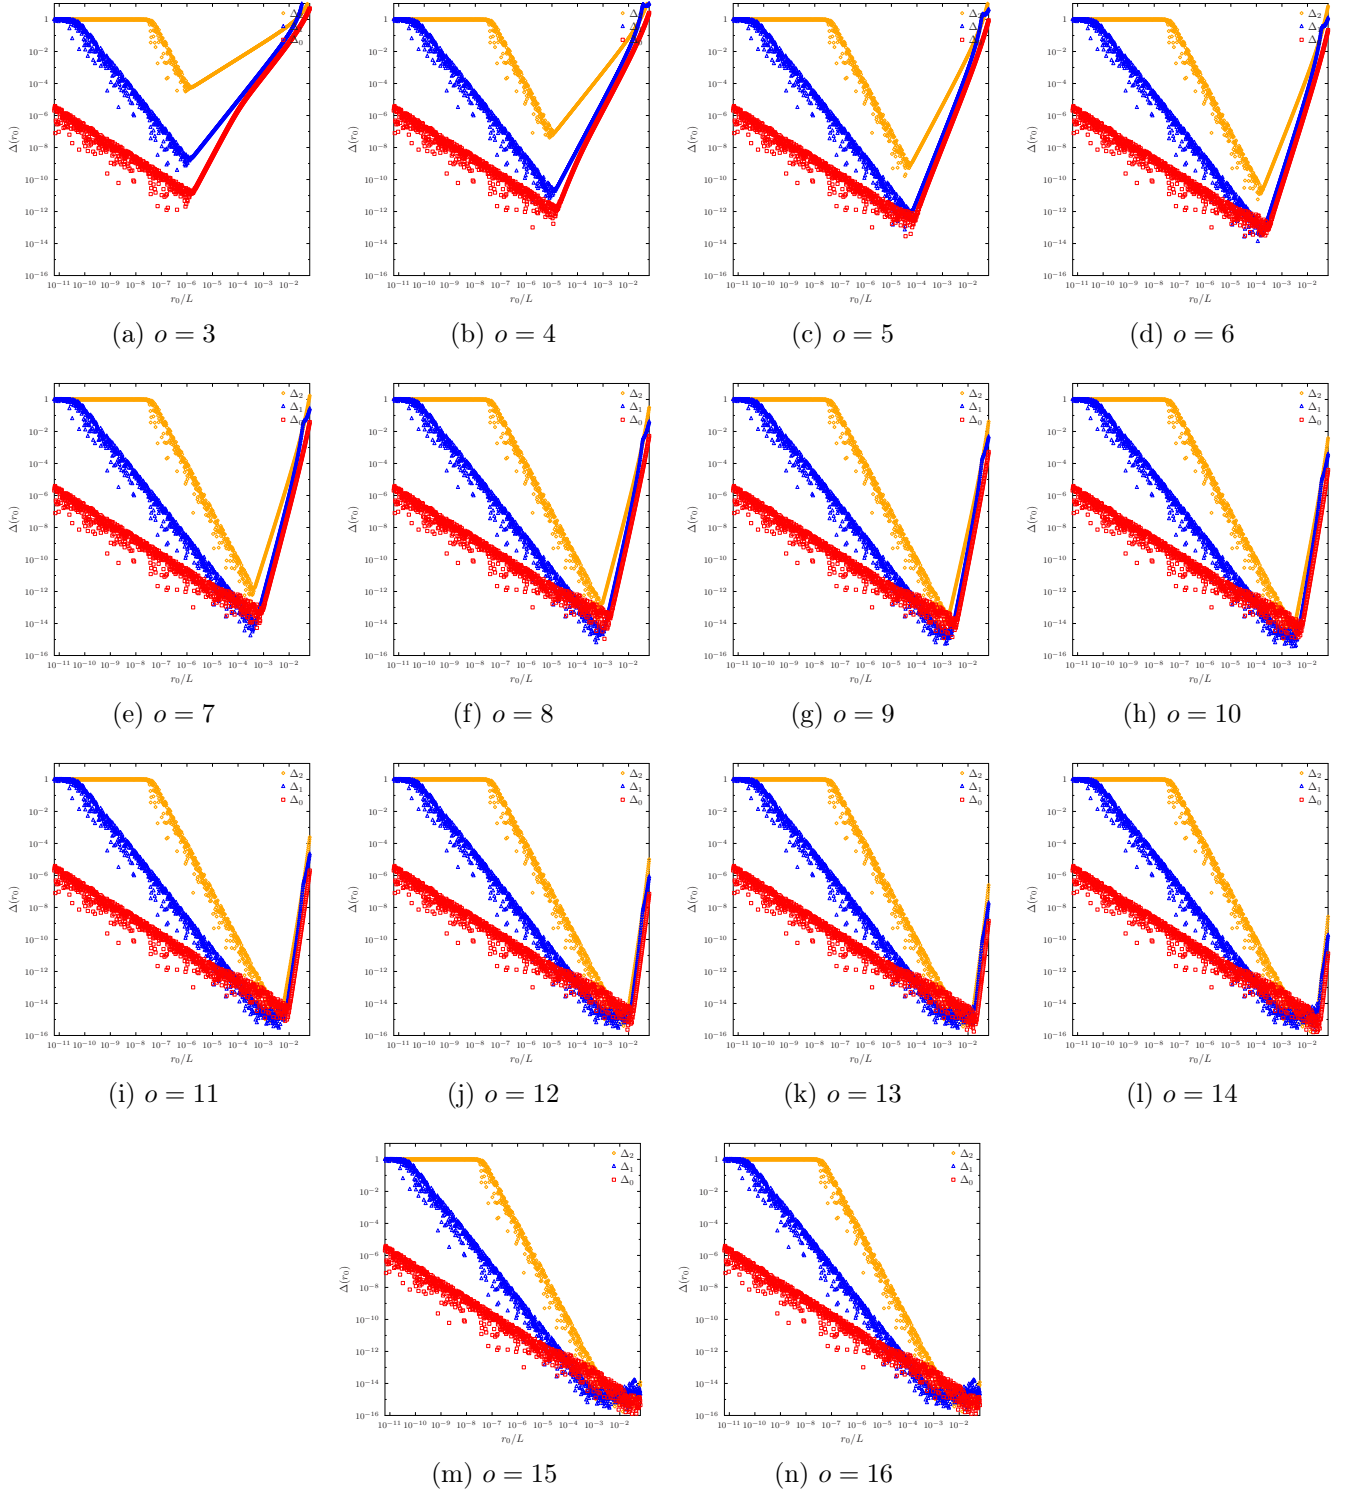

Figure S2: Error  $\Delta$  in Taylor expansion as a function of the switching radius  $R$  for various orders  $o$  of the Taylor expansion, for a 8-node HIP basis with 5 elements; the first non-nuclear node is at  $r_2/L \approx 0.064130$ . Convergence is reached at  $o = 15$ , matching the polynomial order of the 8-node HIP basis.

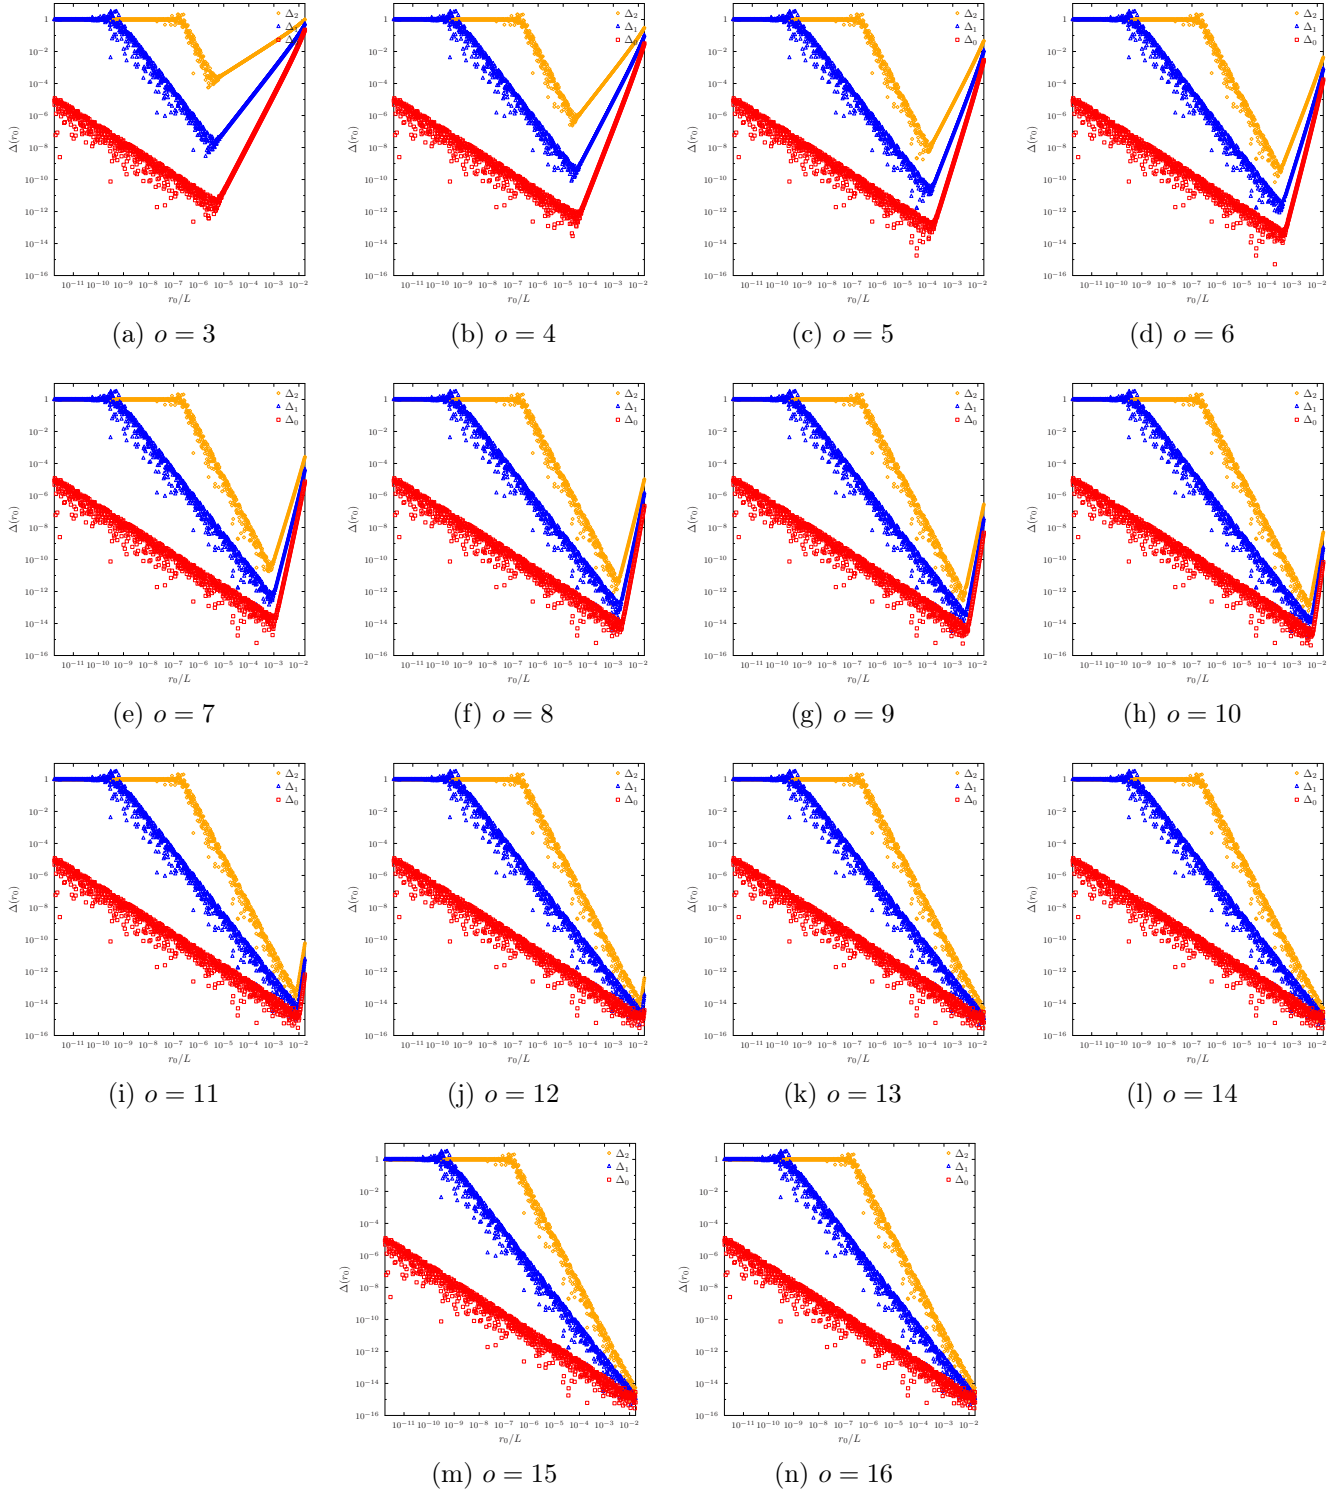

Figure S3: Error  $\Delta$  in Taylor expansion as a function of the switching radius  $R$  for various orders  $o$  of the Taylor expansion, for a 15-node LIP basis with 5 elements; the first non-nuclear node is at  $r_2/L \approx 0.017377$ . Convergence is reached at  $o = 14$ , matching the polynomial order of the 15-node LIP basis.

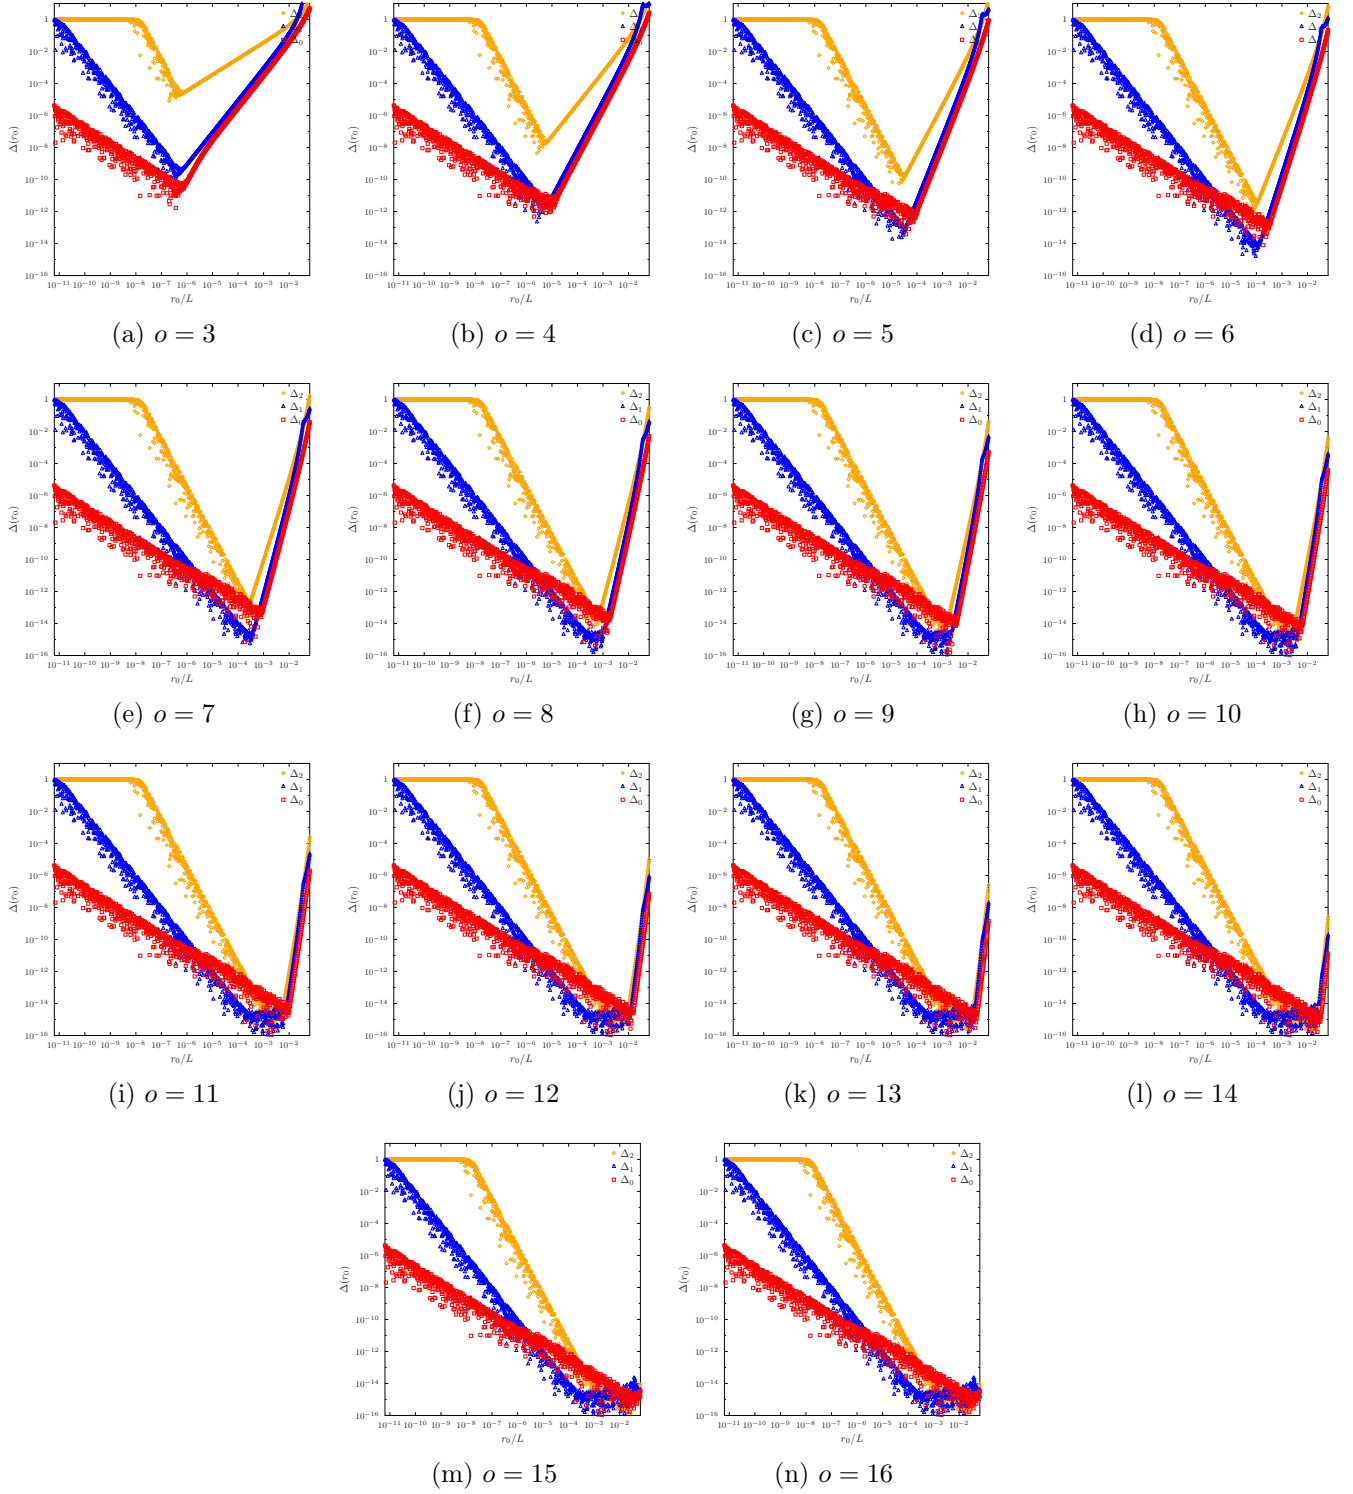

Figure S4: Error  $\Delta$  in Taylor expansion as a function of the switching radius  $R$  for various orders  $o$  of the Taylor expansion, for a 8-node HIP basis with 5 elements; the first non-nuclear node is at  $r_2/L \approx 0.064130$ . Convergence is reached at  $o = 15$ , matching the polynomial order of the 8-node HIP basis.

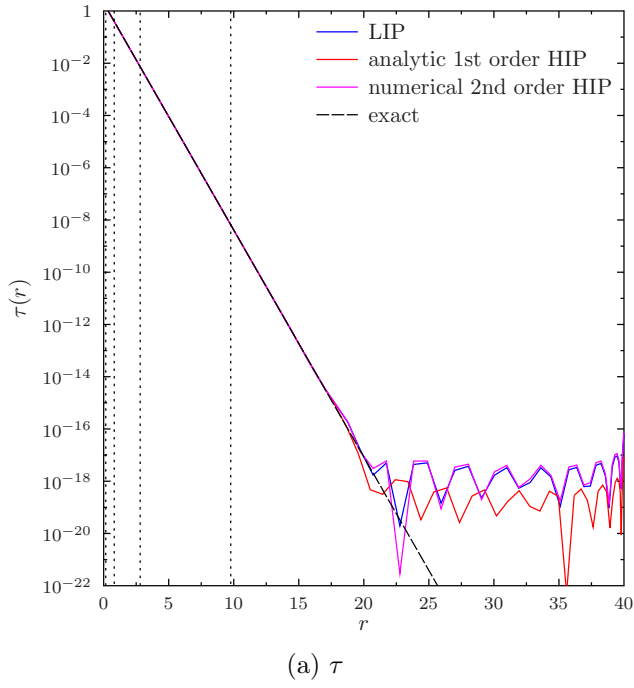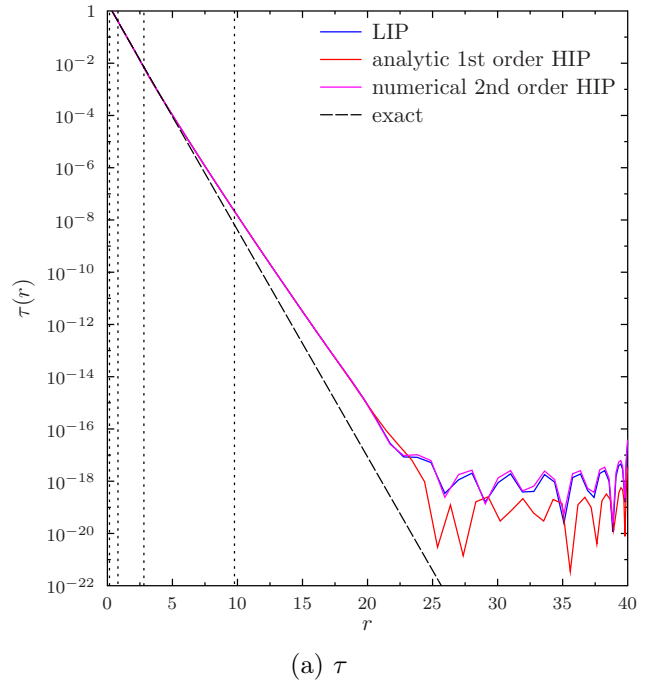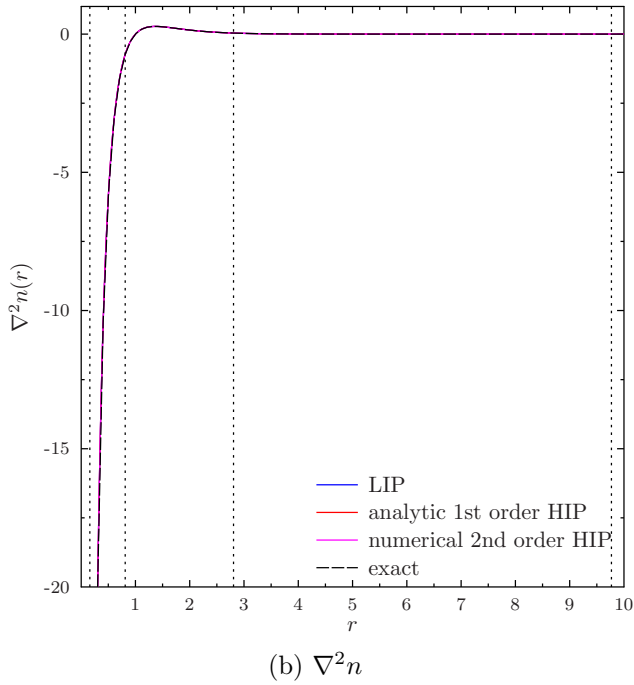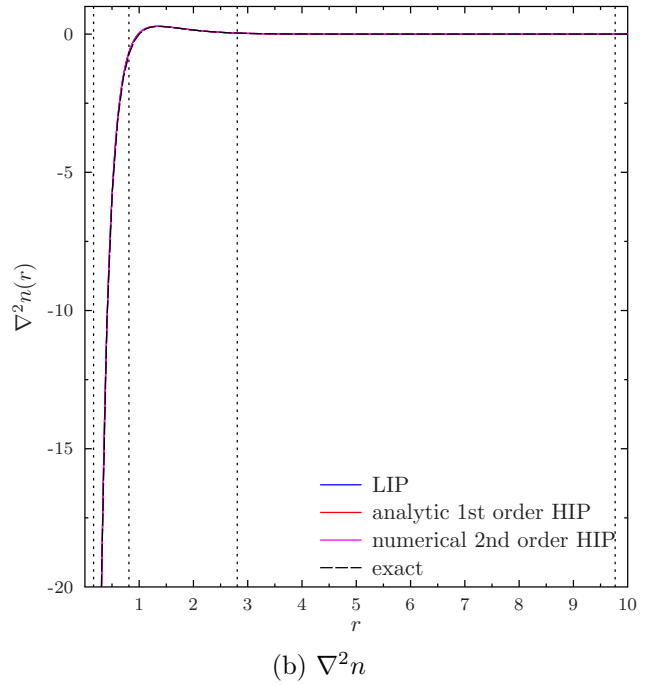

Figure S5:  $\tau$  and  $\nabla^2 n$  for the HF calculation.

Figure S6:  $\tau$  and  $\nabla^2 n$  for the TPSS calculation.

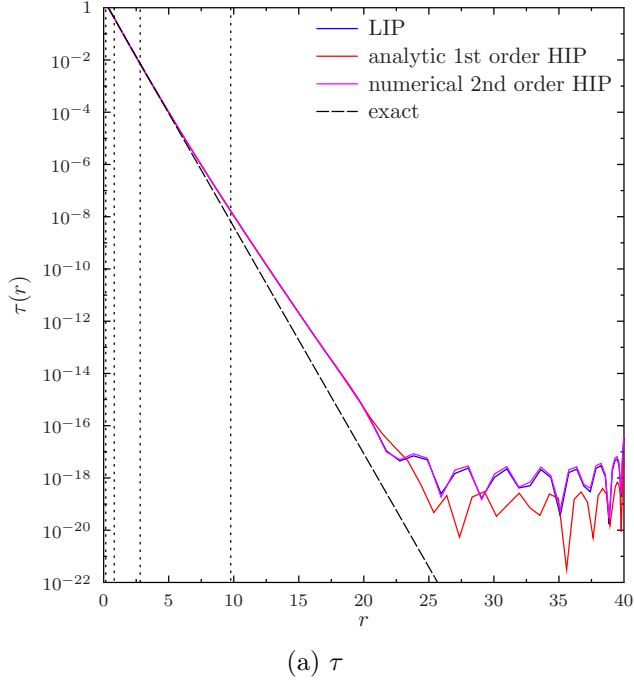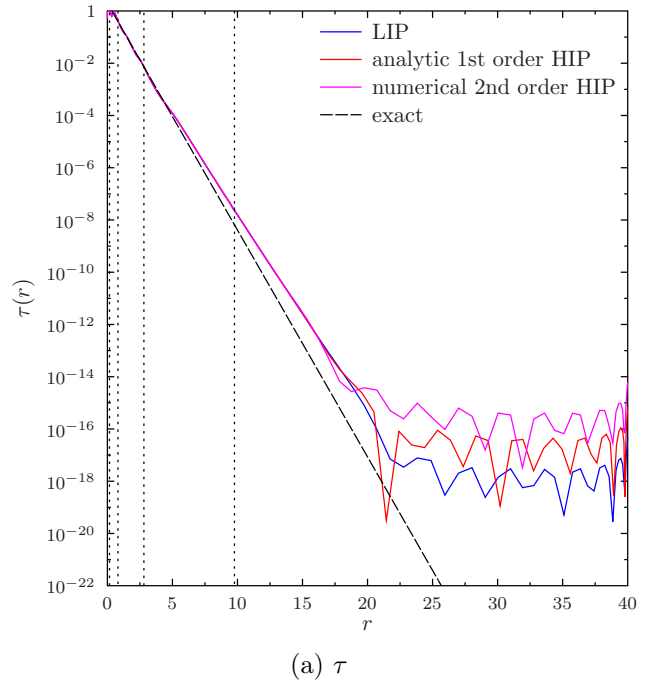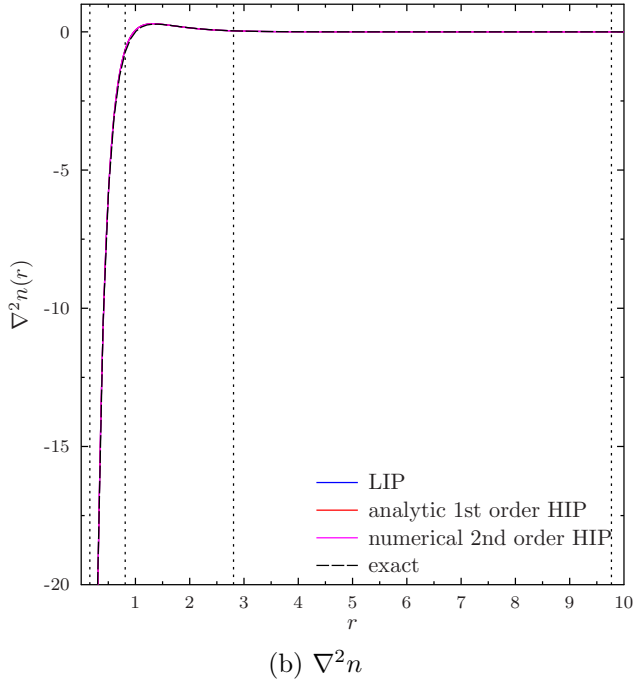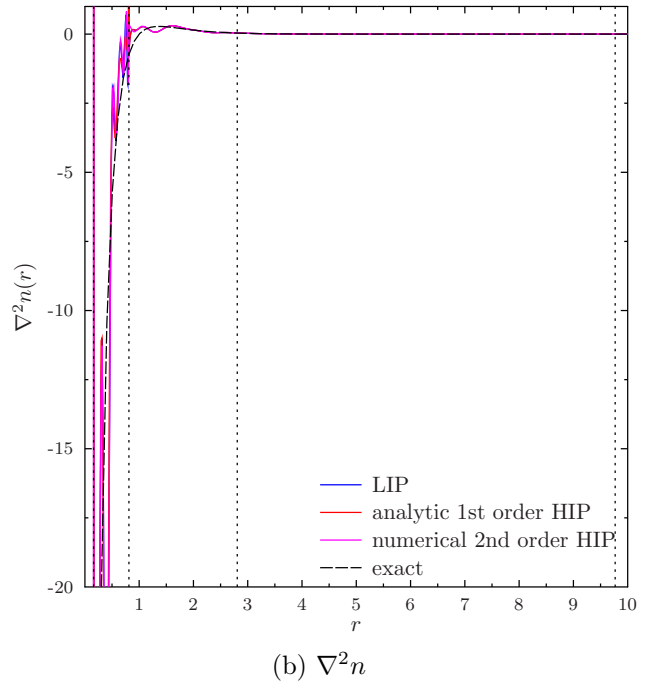

Figure S7:  $\tau$  and  $\nabla^2 n$  for the TASKCC calculation.

Figure S8:  $\tau$  and  $\nabla^2 n$  for the M05 calculation.

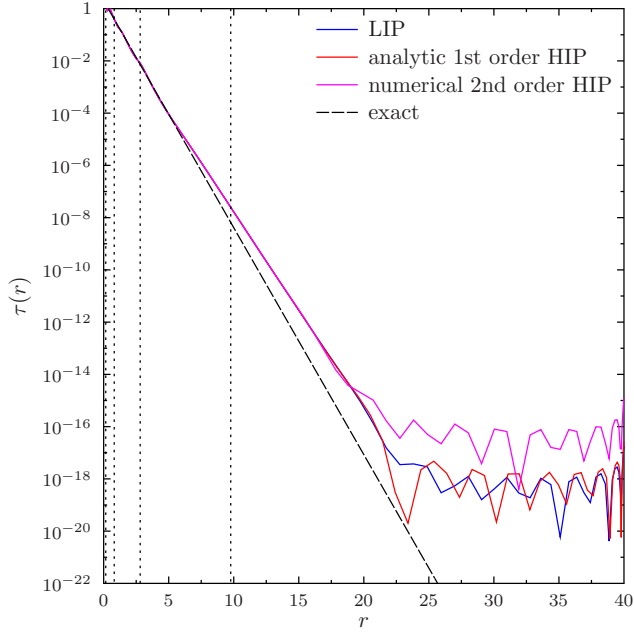

(a)  $\tau$

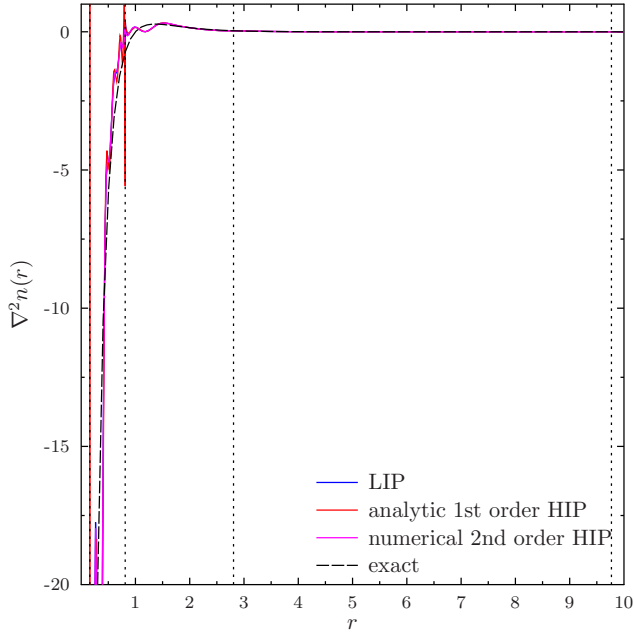

(b)  $\nabla^2 n$

Figure S9:  $\tau$  and  $\nabla^2 n$  for the M06 calculation.

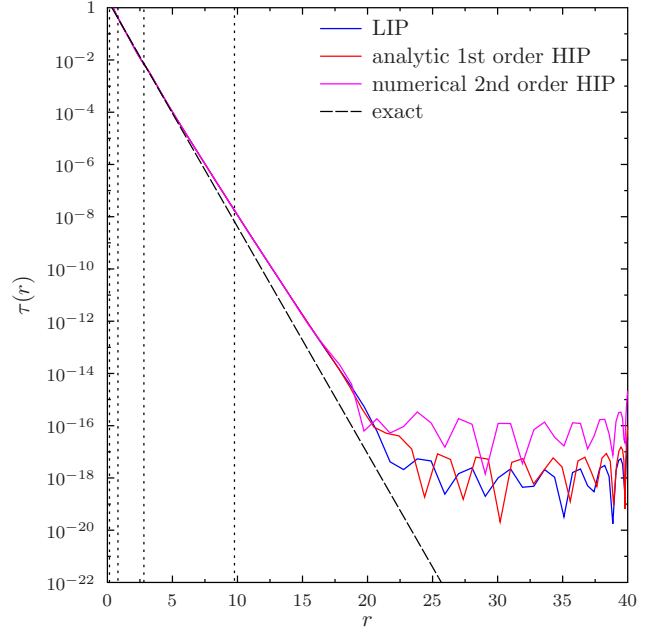

(a)  $\tau$

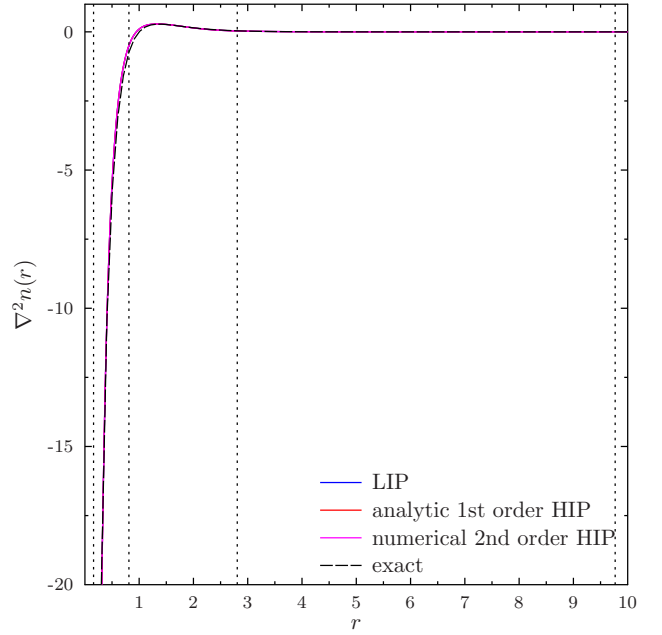

(b)  $\nabla^2 n$

Figure S10:  $\tau$  and  $\nabla^2 n$  for the M06-SX calculation.

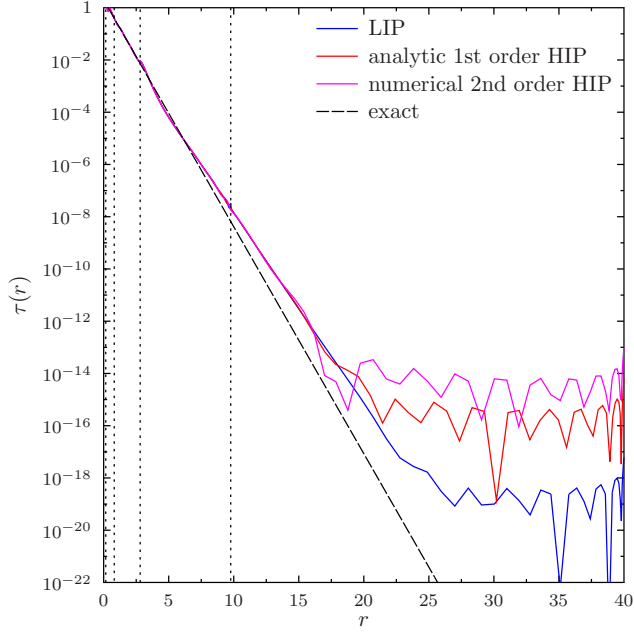

(a)  $\tau$

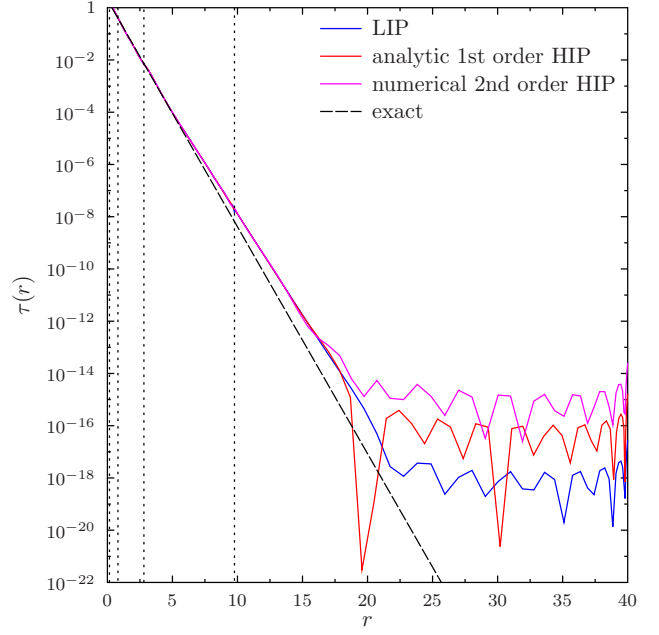

(a)  $\tau$

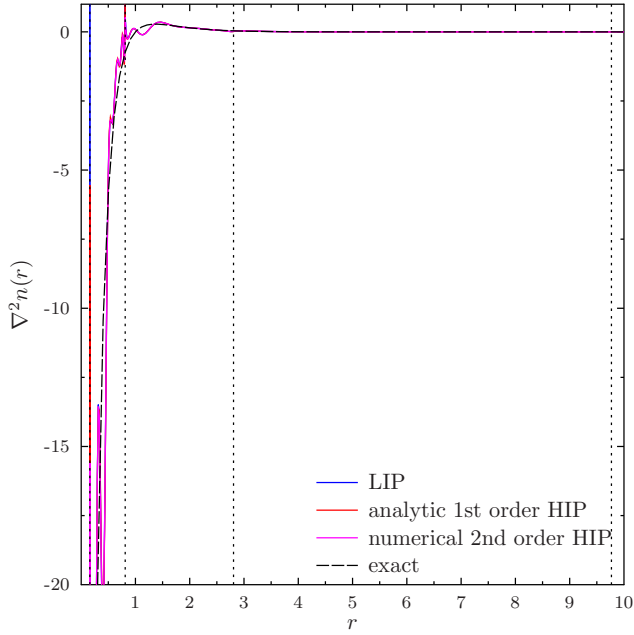

(b)  $\nabla^2 n$

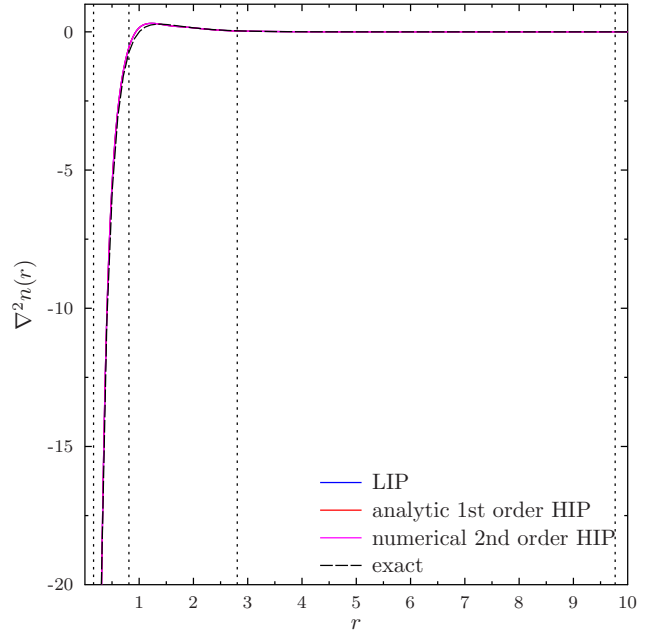

(b)  $\nabla^2 n$

Figure S11:  $\tau$  and  $\nabla^2 n$  for the M06-L calculation.

Figure S12:  $\tau$  and  $\nabla^2 n$  for the revM06 calculation.

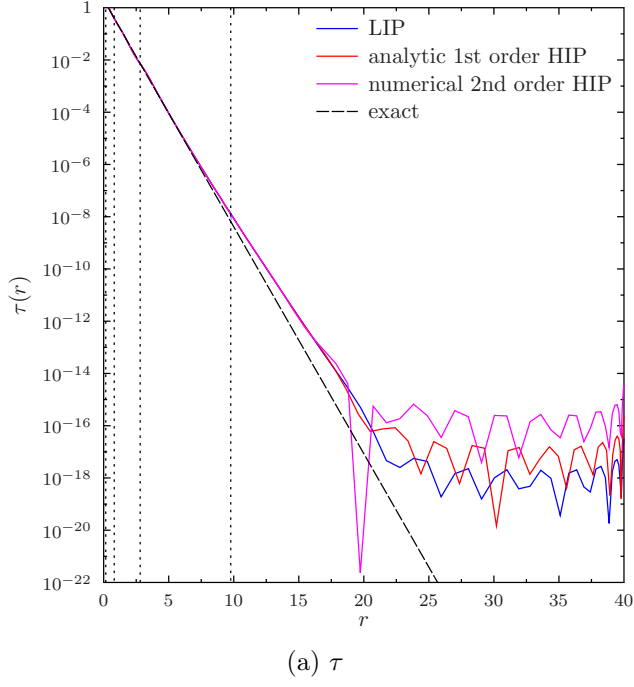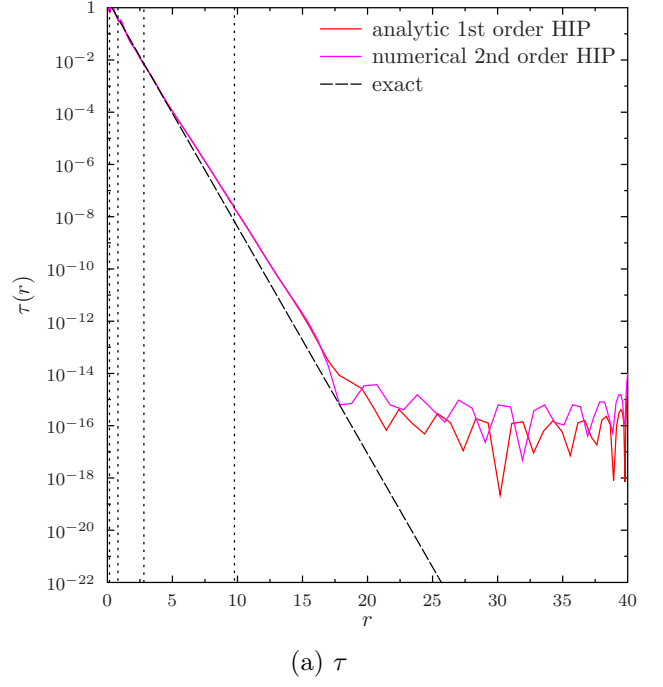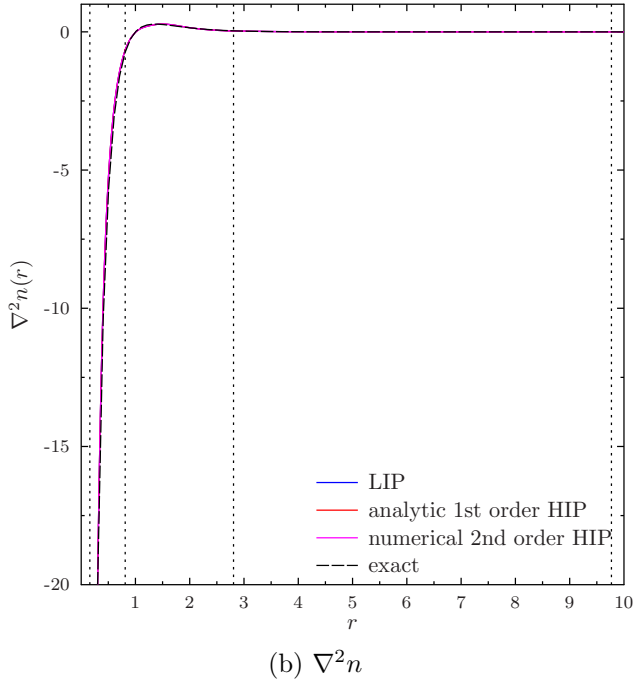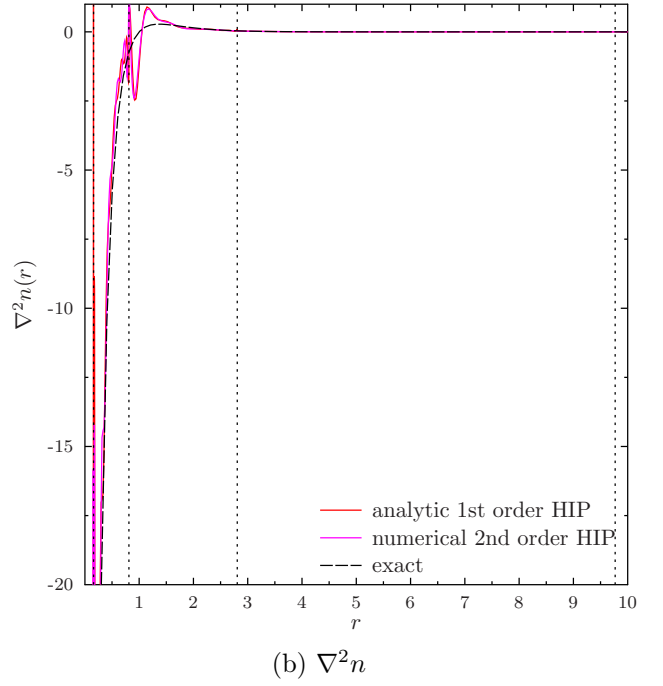

Figure S13:  $\tau$  and  $\nabla^2 n$  for the revM06-L calculation.

Figure S14:  $\tau$  and  $\nabla^2 n$  for the M08-SO calculation.

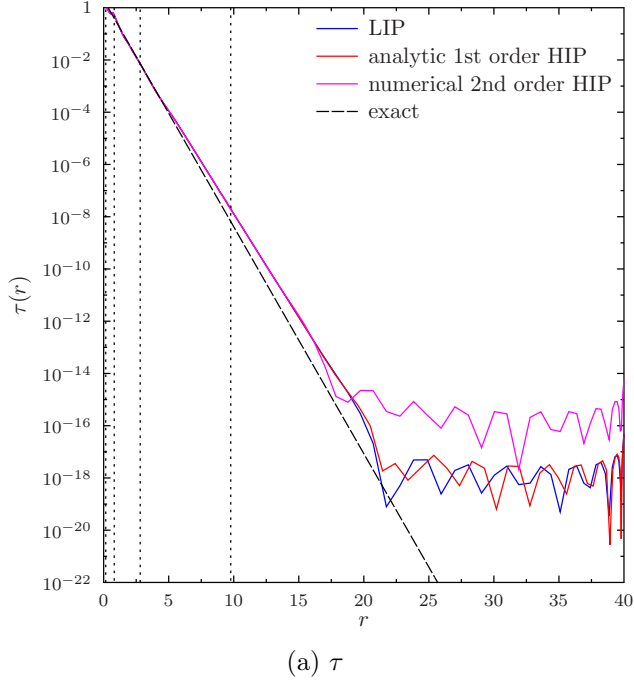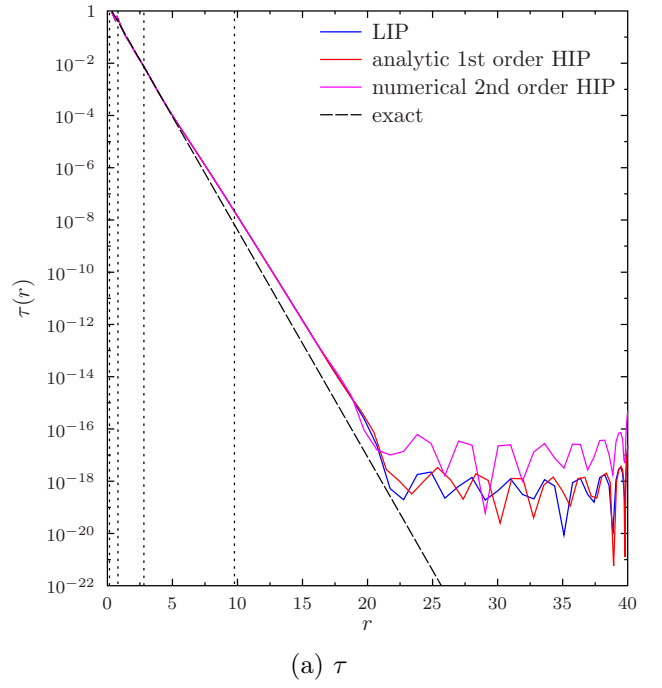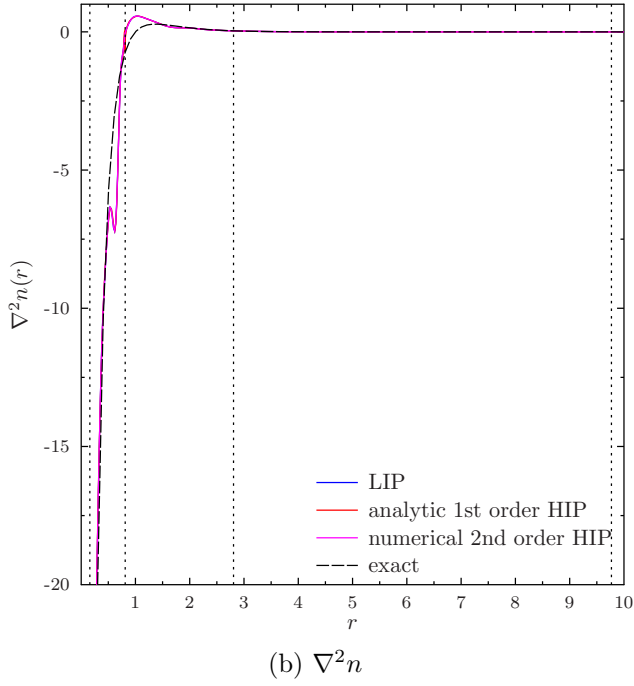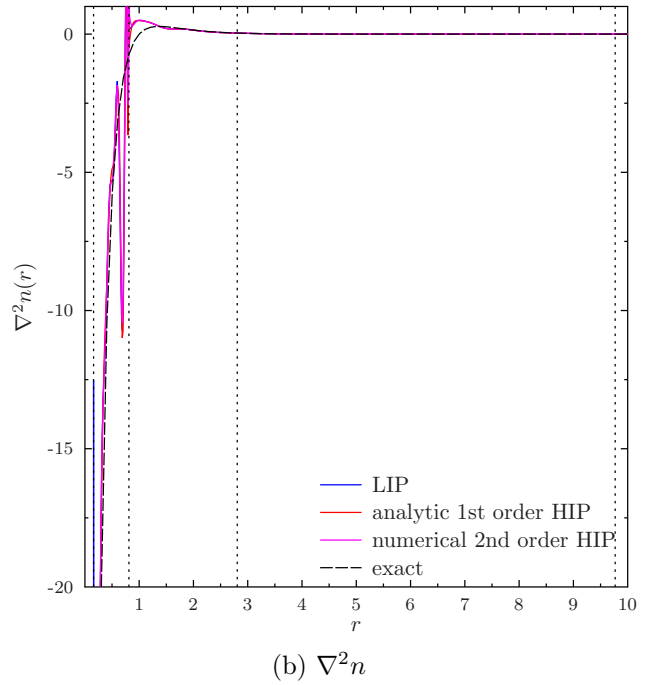

Figure S15:  $\tau$  and  $\nabla^2 n$  for the M08-HX calculation.

Figure S16:  $\tau$  and  $\nabla^2 n$  for the M11 calculation.

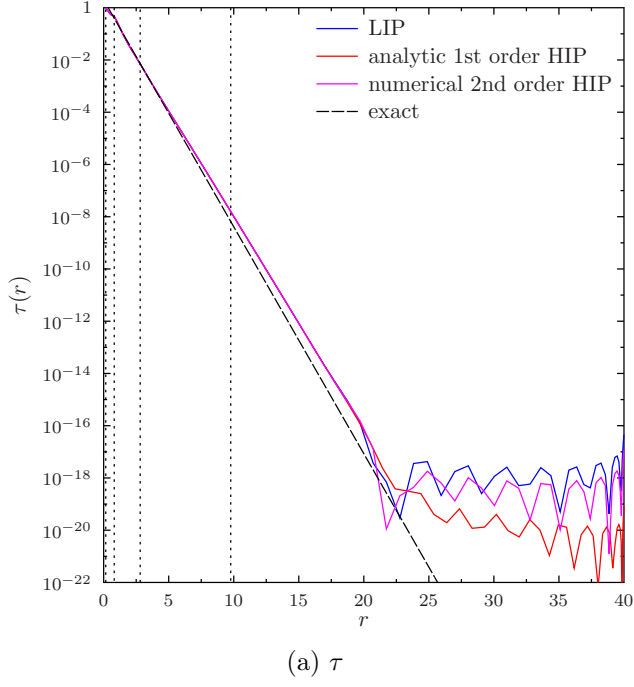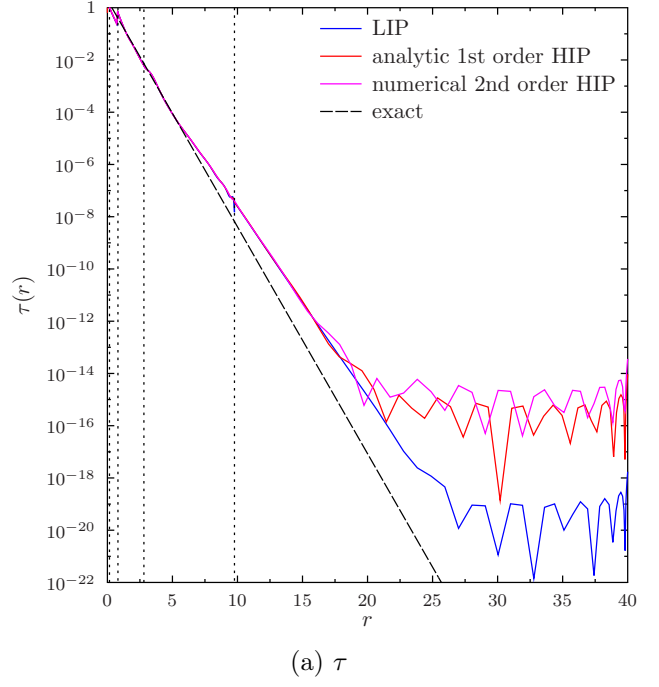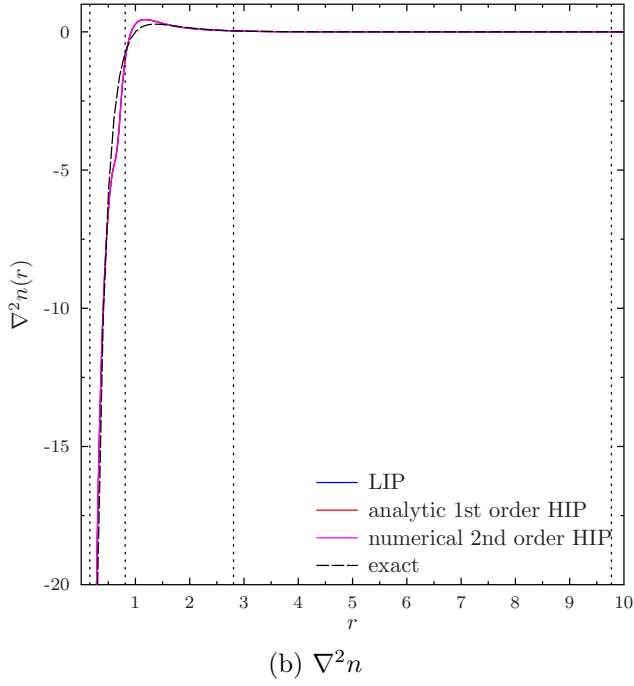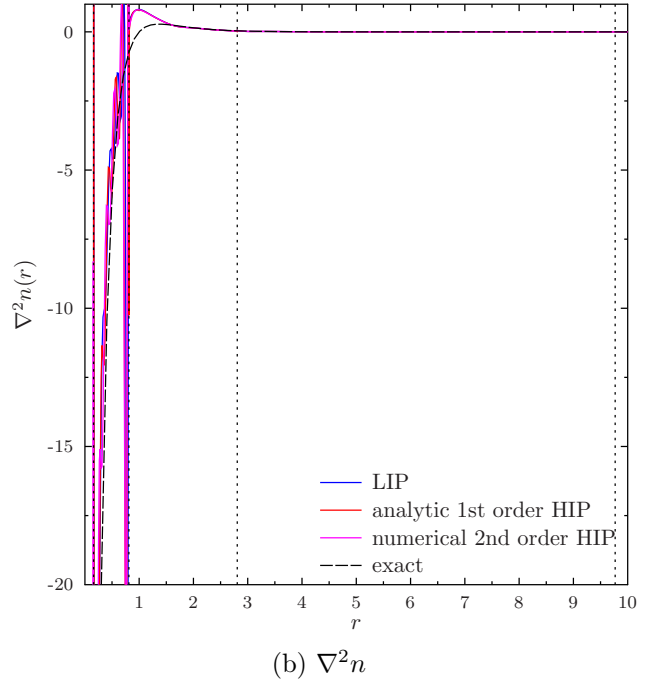

Figure S17:  $\tau$  and  $\nabla^2 n$  for the revM11 calculation.

Figure S18:  $\tau$  and  $\nabla^2 n$  for the M11-L calculation.

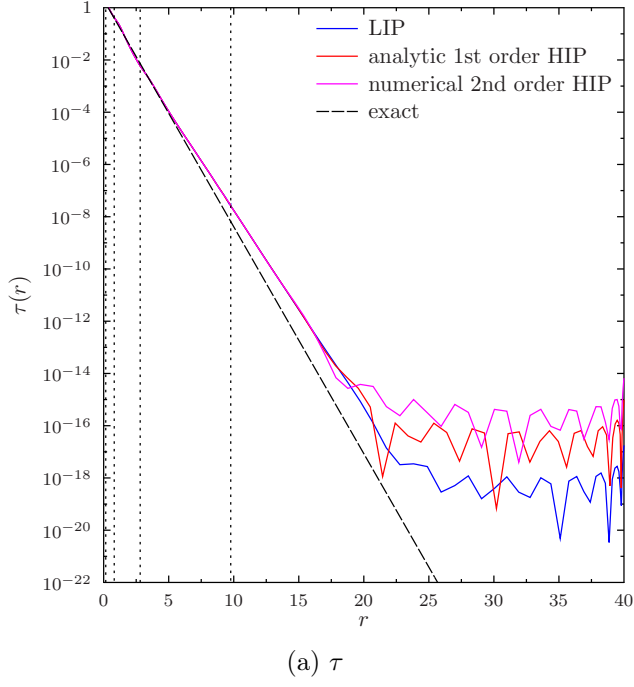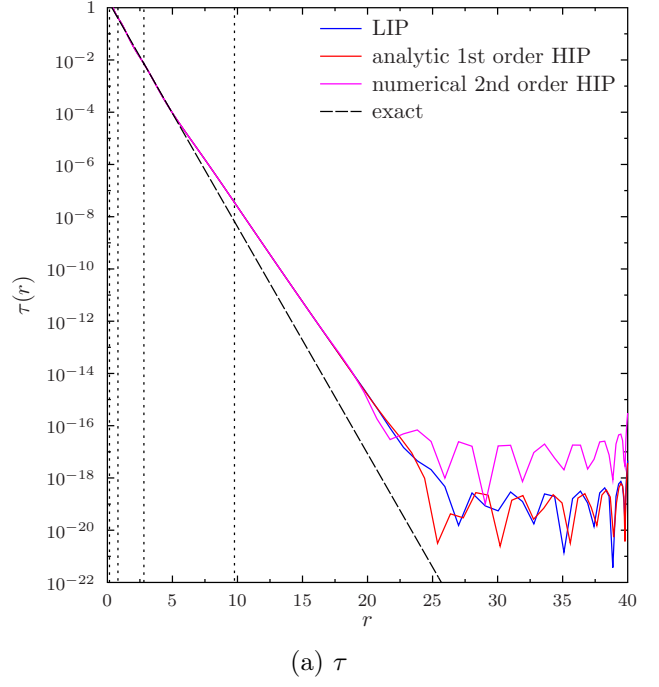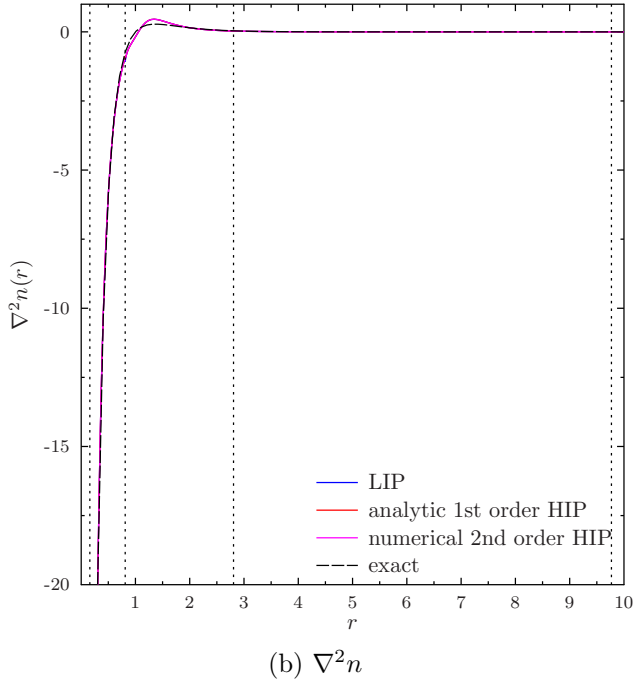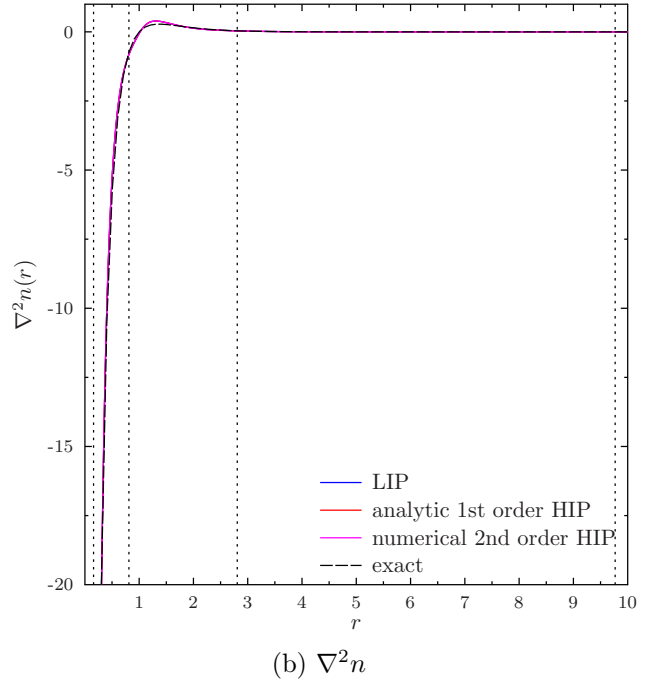

Figure S19:  $\tau$  and  $\nabla^2 n$  for the MN12-SX calculation.

Figure S20:  $\tau$  and  $\nabla^2 n$  for the MN12-L calculation.

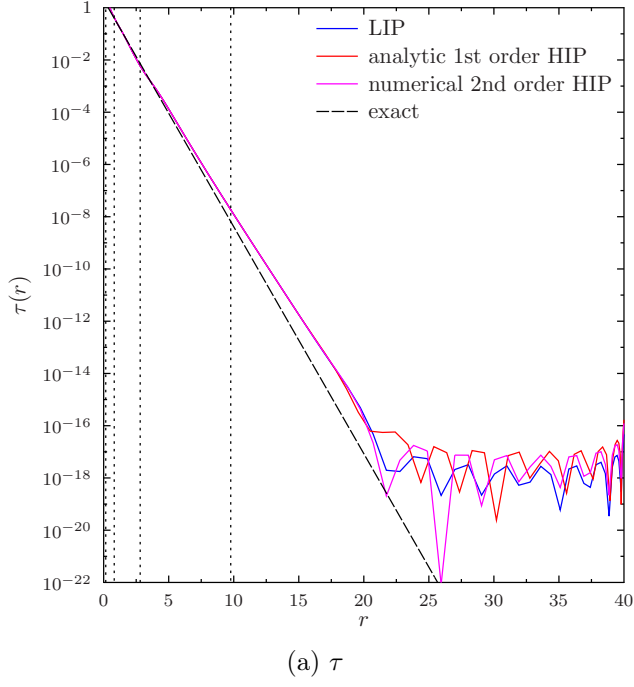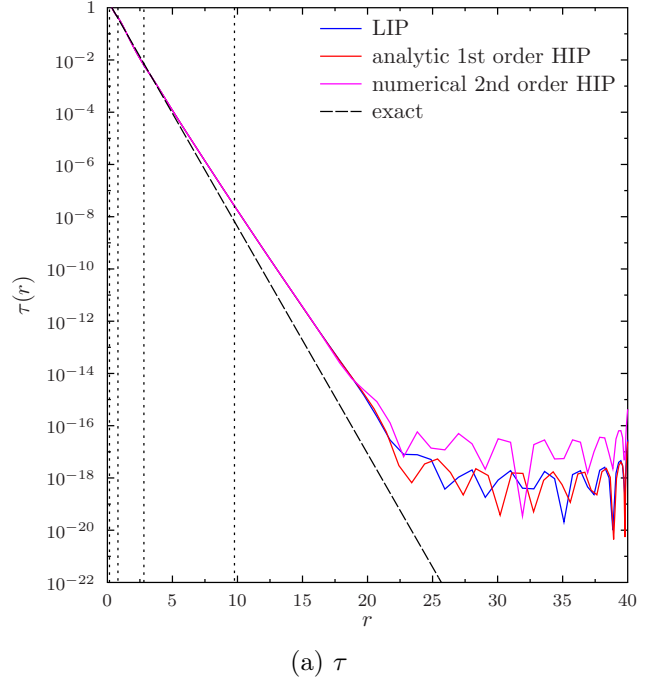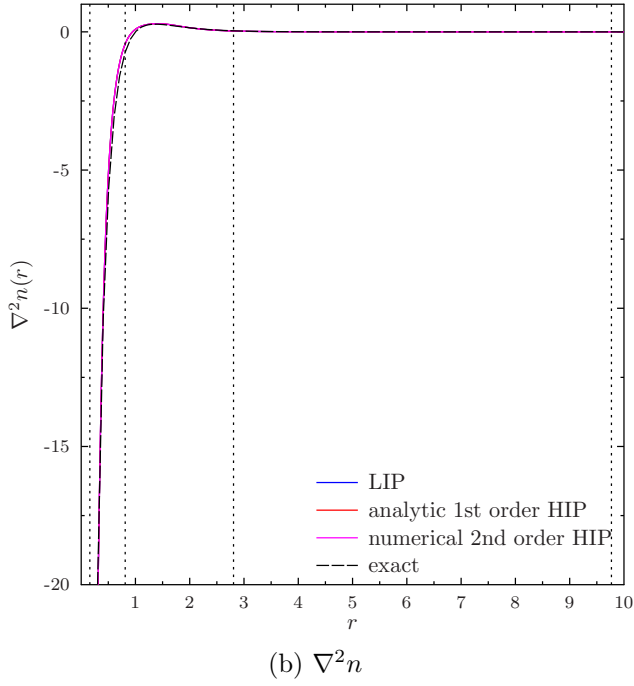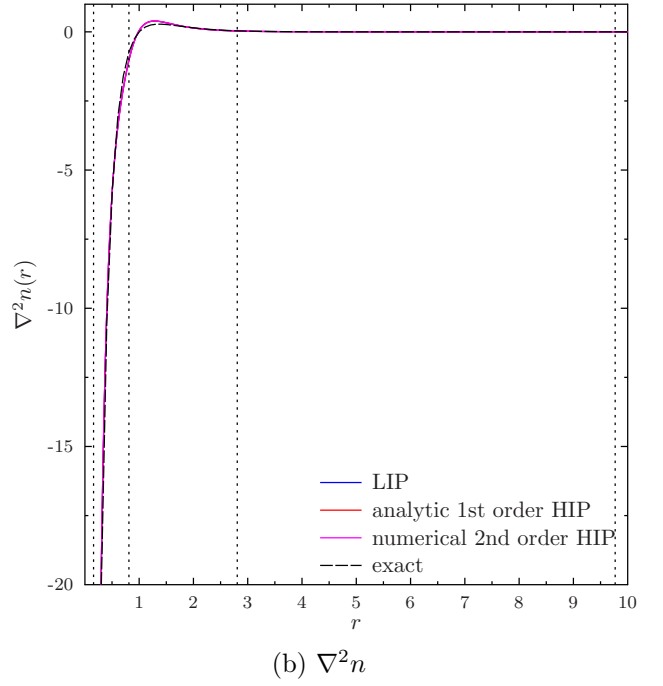

Figure S21:  $\tau$  and  $\nabla^2 n$  for the MN15 calculation.

Figure S22:  $\tau$  and  $\nabla^2 n$  for the MN15-L calculation.

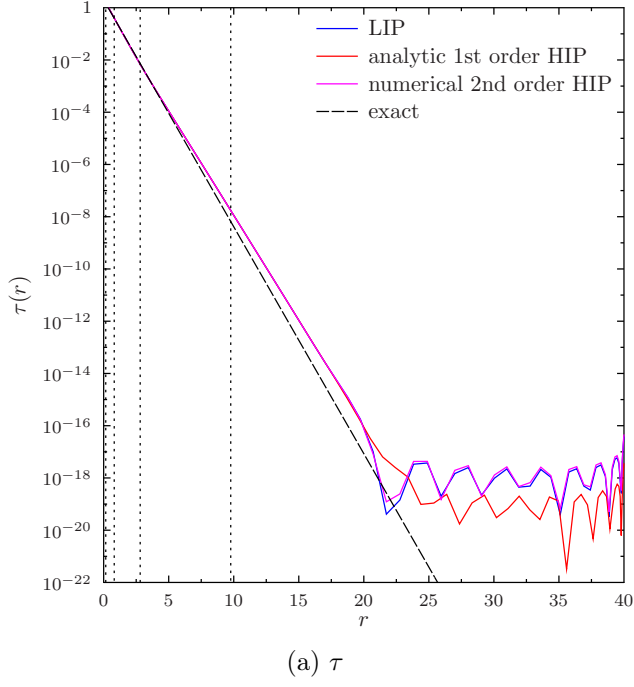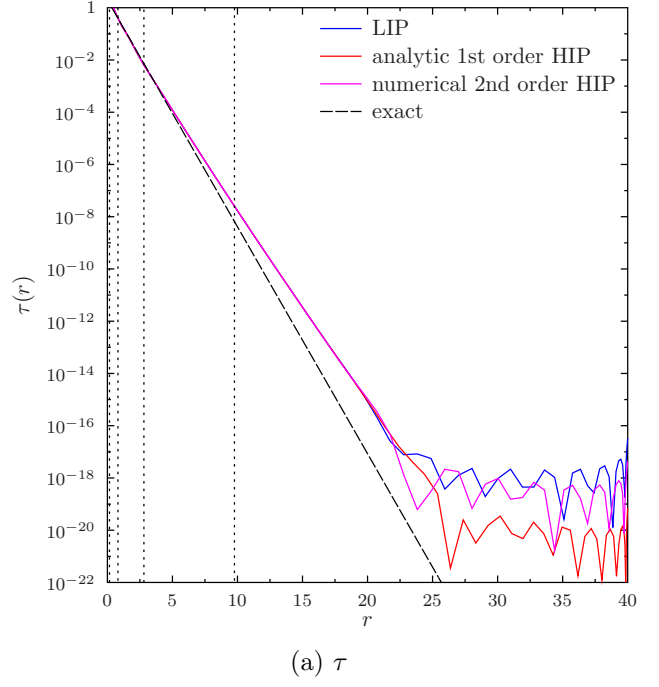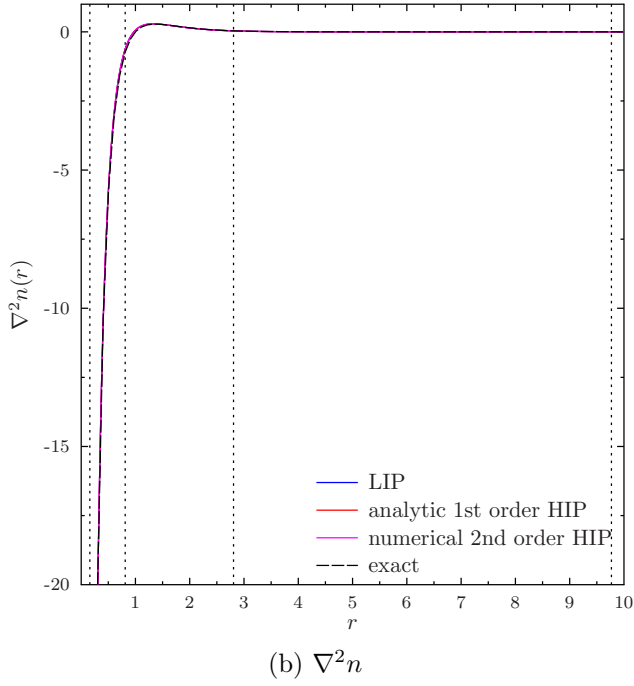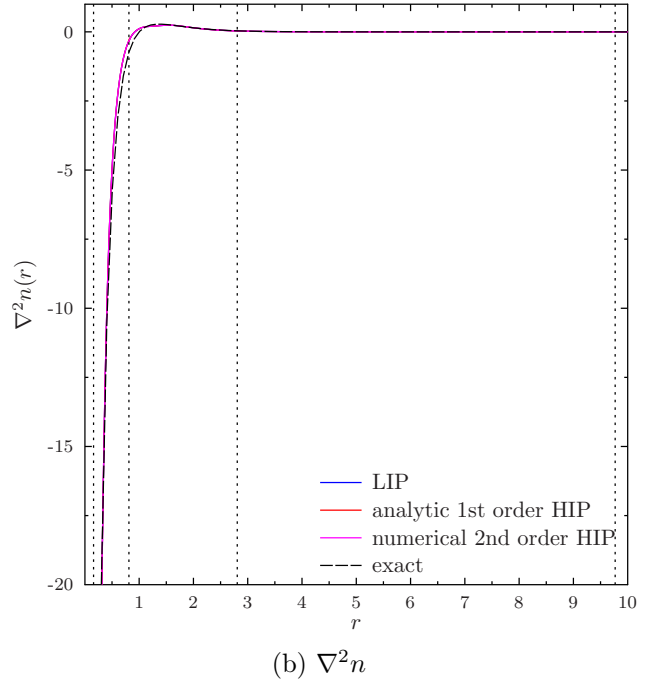

Figure S23:  $\tau$  and  $\nabla^2 n$  for the  $\omega$ B97X-noV calculation.

Figure S24:  $\tau$  and  $\nabla^2 n$  for the B97M-noV calculation.

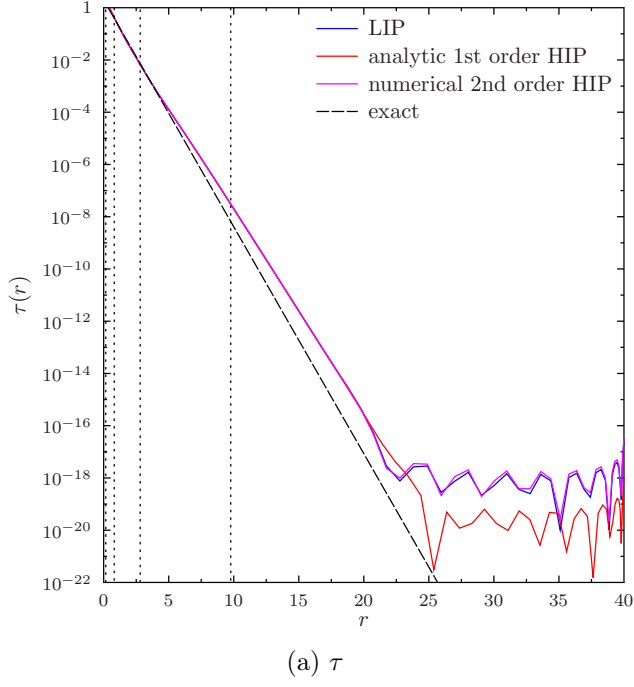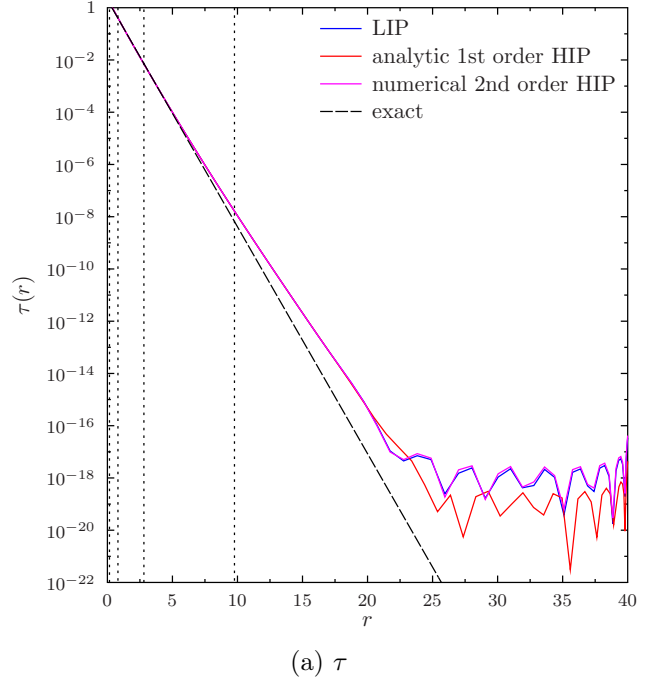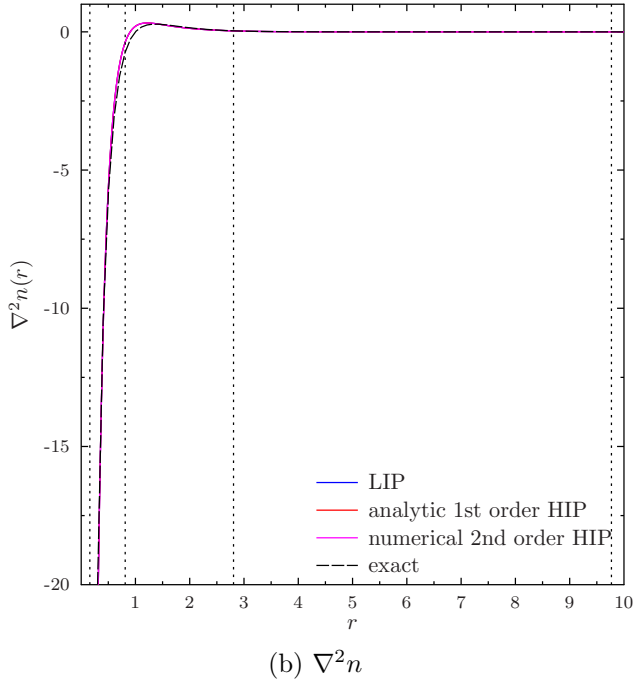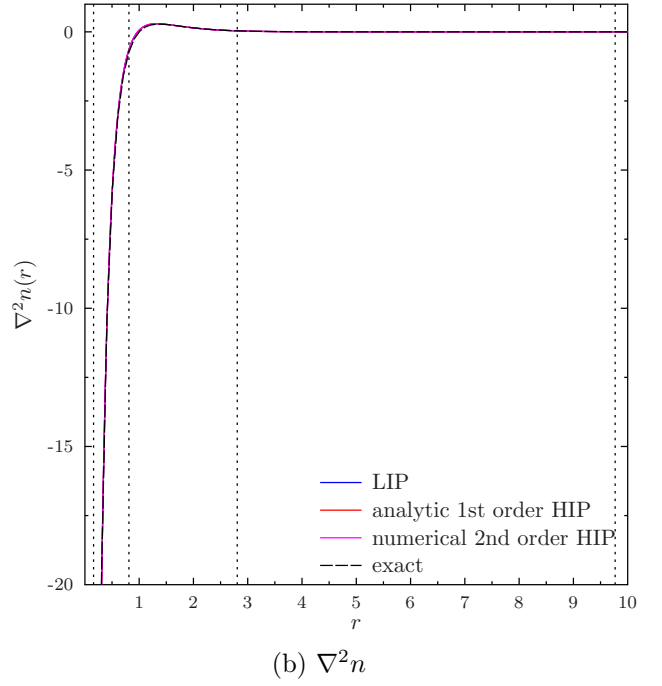

Figure S25:  $\tau$  and  $\nabla^2 n$  for the  $\omega$ B97M-noV calculation.

Figure S26:  $\tau$  and  $\nabla^2 n$  for the  $r^2$ SCAN calculation.
